# Supplementary material for: Phase separation dynamics in deformable droplets
Source: arXiv:2111.04655 ancillary file (2021-11-08)
Supplement: Supplementary file 1 [file SI.pdf]

# Supplementary Information
# Symmetry-breaking dynamics of unmixing droplets

Simon Gsell[a,b], Matthias Merkel[b]

[a] Aix Marseille Univ, CNRS, IBDM (UMR 7288), Turing Centre for Living systems, Marseille, France
[b] Aix Marseille Univ, Université de Toulon, CNRS, CPT (UMR 7332), Turing Centre for Living systems, Marseille, France

# 1 Numerical methods

## 1.1 Hydrodynamics

The hydrodynamics equations (equations (6a) and (6b) in the paper) are integrated using a lattice-Boltzmann approach[1]. The method relies on a mesoscopic description of the material dynamics. It is based on a particle distribution function $f(\boldsymbol{x}, \boldsymbol{\xi}, t)$, which represents the density of fluid particles with velocity $\boldsymbol{\xi}$ at location $\boldsymbol{x}$ and time $t$. Its dynamics is governed by the Boltzmann equation,

$$\frac{\partial f}{\partial t} + \boldsymbol{\xi} \cdot \boldsymbol{\nabla_x f} + \frac{1}{\rho}\boldsymbol{F} \cdot \boldsymbol{\nabla_\xi f} = \Omega(f), \tag{S1}$$

where $\nabla_x \equiv (\partial/\partial x, \partial/\partial y)$ is the spatial gradient operator, $\nabla_\xi \equiv (\partial/\partial \xi_x, \partial/\partial \xi_y)$ is the gradient operator in the velocity space, $\boldsymbol{F}$ is the external body force (related to the phase-field model in the present work), $\rho$ is the fluid density and $\Omega$ designates the collision operator. At the macroscopic level, it can be shown that the Boltzmann equation is equivalent to the Navier-Stokes equations.

The discretization of Eq. (S1) in velocity space, physical space and time leads to the lattice-Boltzmann equation. The velocity space is discretized on a set of velocity vectors $\{\boldsymbol{c_l},\ l = 0, ..., Q-1\}$, where $Q$ is the number of discrete velocities. In the present work, a $D2Q9$ velocity set is used, i.e. the velocity space is discretized into nine velocity vectors $\boldsymbol{c_l}$, which are

$$\boldsymbol{c_l} = \begin{cases} (0,0), & l = 0, \\ c\left(\cos(\frac{\pi(l-1)}{2}), \sin(\frac{\pi(l-1)}{2})\right), & l \in [1,4], \\ \sqrt{2}c\left(\cos(\frac{\pi(2l-9)}{4}), \sin(\frac{\pi(2l-9)}{4})\right), & l \in [5,8], \end{cases} \tag{S2}$$

where $c$ is the lattice speed. The particle densities at velocities $\{\boldsymbol{c_l}\}$ are represented by the discrete-velocity distribution functions $\{f_l(\boldsymbol{x}, t)\}$, also called particle populations. Time and space are discretized so that particle populations are transported from one node to a neighboring one during one time step, namely $\Delta x/\Delta t = \Delta y/\Delta t = c$. The associated grid is thus Cartesian and uniform, with $\Delta x = \Delta y$. Within this section, all quantities are normalized by $c$ and $\Delta t$, so that $\Delta x = \Delta t = 1$.

Using this normalization, the lattice-Boltzmann equation reads

$$f_l(\boldsymbol{x} + \boldsymbol{c_l}, t+1) - f_l(\boldsymbol{x}, t) = \Omega_l(\boldsymbol{x}, t) + S_l(\boldsymbol{x}, t), \tag{S3}$$

where $\Omega_l$ is the discretized collision operator and $S_l$ is a discrete source term related to the macroscopic body force. The left-hand side of (S3) is called the streaming operation; the right-hand side is the collision process. Equation (S3) is explicit and the streaming and collision can be treated separately at each time step.

The macroscopic flow quantities are moments of the particle populations in the velocity space. In particular, the density $\rho$ and the fluid momentum $\rho \boldsymbol{u}$ read

$$\rho_m = \sum_{l=0}^{8} f_l, \qquad \rho_m \boldsymbol{u} = \sum_{l=0}^{8} f_l \boldsymbol{c_l} + \frac{1}{2}\boldsymbol{F}. \tag{S4}$$

Even though the lattice-Boltzmann method allows small variations of the fluid density, in practice these variations are negligible if the flow velocity remains small enough; the fluid can thus be considered as nearly incompressible.

The collision operator typically consists of a relaxation of particle distributions towards an equilibrium distribution. In the present simulation, a two-relaxation-time collision operator is employed [2,3], namely

$$\Omega_l = -\frac{1}{\tau^+}\left(f_l^+ - f_l^{eq+}\right) - \frac{1}{\tau^-}\left(f_l^- - f_l^{eq-}\right), \tag{S5}$$

where symmetric populations $f_l^+ = (f_l + f_{\bar{l}})/2$ and anti-symmetric populations $f_l^- = (f_l - f_{\bar{l}})/2$, with the symmetric index $\bar{l}$ defined as $\boldsymbol{c}_{\bar{l}} = -\boldsymbol{c}_l$, are relaxed through two distinct relaxation times $\tau^+$ and $\tau^-$. The symmetric and anti-symmetric equilibrium distributions are defined as $f_l^{eq+} = (f_l^{eq} + f_{\bar{l}}^{eq})/2$ and $f_l^{eq-} = (f_l^{eq} - f_{\bar{l}}^{eq})/2$, with

$$f_l^{(eq)} = w_l \rho \left(1 + \frac{\boldsymbol{u}\cdot\boldsymbol{c}_l}{c_s^2} + \frac{(\boldsymbol{u}\cdot\boldsymbol{c}_l)^2}{2c_s^4} - \frac{\boldsymbol{u}\cdot\boldsymbol{u}}{2c_s^2}\right). \tag{S6}$$

The weights $\{w_l\}$ are specific to the velocity set. In the present case ($D2Q9$ velocity set), $w_0 = 4/9$, $w_1 = w_2 = w_3 = w_4 = 1/9$ and $w_5 = w_6 = w_7 = w_8 = 1/36$. The symmetric relaxation time $\tau^+$ is related to the macroscopic dynamic viscosity through $\eta = \rho c_s^2(\tau^+ - 1/2)$, while $\tau^-$ is a free numerical parameter. In order to avoid viscosity-dependent numerical errors, the parameter $\Lambda_\tau = (\tau^+ - 1/2)(\tau^- - 1/2)$ is fixed to 1/6. In the present simulations, the fluid viscosity varies at the droplet interface; therefore, the value of $\tau^-$ is varied dynamically to keep $\Lambda_\tau$ constant.

The source term $S_l$ is based on the scheme proposed by Guo et al. [4] adapted to the two-relaxation time framework:

$$S_l = w_l \left[\frac{\boldsymbol{c}_l - \boldsymbol{u}}{c_s^2} + \frac{(\boldsymbol{c}_l\cdot\boldsymbol{u})\cdot\boldsymbol{c}_l}{c_s^4}\right]\cdot\boldsymbol{F}. \tag{S7}$$

One can show based on a Chapman-Enskog analysis that in the limit of small fluid velocities $|\boldsymbol{u}| \ll c_s$, the Boltzmann equation (S1) is equivalent to the incompressible Navier-Stokes equations at the macroscopic level [1]. The resulting fluid dynamics thus includes inertial effects. Their magnitude is controlled by the Reynolds number $Re = \rho|\boldsymbol{u}|d/\eta$, where $\rho$ is the fluid density, $d$ is the typical length scale of the flow and $\eta$ is the dynamic viscosity. We keep $Re$ small enough to avoid inertial effects in the flow. Using a typical surface-tension driven velocity $\sigma_{12}/\eta$ and the droplet diameter $L$, the nominal Reynolds number reads $Re_n = \rho\sigma_{12}L/\eta^2$. In the present simulations, $Re_n = 0.1$. The effective Reynolds number $Re_L = \rho|\boldsymbol{u}|L/\eta$ has been systematically monitored during the simulations. In practice, $Re_L$ remains always lower than 0.1.

## 1.2 Phase-field dynamics

The phase-field dynamics (equations (5a) and (5b) in the paper) are simulated using a finite-volume method. The method is illustrated for the $\phi$-field dynamics in the following. Considering any closed volume $\Omega_k$ in the physical space $\Omega$, the integral form of the $\phi$-field conservation equation reads, in two dimensions,

$$\int_{\Omega_k} \frac{\partial\phi}{\partial t} dS + \int_{\Omega_k} \nabla\cdot(\boldsymbol{u}\phi) dS = \int_{\Omega_k} \nabla\cdot\left[(1-\psi)\Gamma_\phi \nabla\mu_\phi\right] dS. \tag{S8}$$

Using the divergence theorem, the $\phi$-field conservation becomes a flux balance at the interface $\partial\Omega_k$ of the considered volume, namely

$$\int_{\Omega_k} \frac{\partial\phi}{\partial t} dS = -\oint_{\partial\Omega_k} \phi\boldsymbol{u}\cdot\boldsymbol{dl} + \oint_{\partial\Omega_k} (1-\psi)\Gamma_\phi \nabla\mu_\phi\cdot\boldsymbol{dl}, \tag{S9}$$

where $\boldsymbol{dl}$ is the outwards unit vector at the boundary $\partial\Omega_k$.

Considering a regular and Cartesian mesh, the physical space is discretized through a series of square domains $\Omega_{ij}$ with volumes $V_{ij}$, where $i$ and $j$ denote indices along the $x$ and $y$ directions. The volume-averaged $\phi$-field in each volume is denoted by $\phi_{ij}$. The finite-volume mesh is chosen so that the center of the volumes match the lattice-Boltzmann nodes; therefore, the discrete phase fields are expressed at the same locations as the discrete fluid velocity and pressure. In each volume, the $\phi$-field conservation equation can be expressed as

$$\frac{\partial \phi_{ij}}{\partial t} V_{ij} = \sum_{k_{ij}} F_{k_{ij}} = \sum_{k_{ij}} (F_{Ak_{ij}} + F_{Dk_{ij}}), \tag{S10}$$

where $k_{ij} \in \{S_{ij}, E_{ij}, N_{ij}, W_{ij}\}$ denote the four boundaries (South, East, North, West) of the $(i, j)$ cell, and $F_{Ak_{ij}}$ and $F_{Dk_{ij}}$ are the advective and diffusive fluxes integrated on these surfaces. The discrete calculation of these fluxes is illustrated for $k_{ij} = E_{ij}$ hereafter.

The advective flux is equal to $F_{AE_{ij}} = \phi_{E_{ij}} \boldsymbol{u_{E_{ij}}} \cdot \boldsymbol{dl_{E_{ij}}} = \phi_{E_{ij}} u_{E_{ij}}$. The velocity on a cell boundary is obtained through a central averaging, i.e. $u_{E_{ij}} = (u_{ij} + u_{i+1j})/2$. The flux is then computed using a first-order upwind scheme, by setting $\phi_{E_{ij}} = \phi_{ij}$ if $u_{E_{ij}} > 0$ and $\phi_{E_{ij}} = \phi_{i+1j}$ if $u_{E_{ij}} < 0$. The diffusive flux on the east face is expressed as $F_{DE_{ij}} = (1 - \psi_{E_{ij}})\Gamma_\phi (\partial\mu_\phi/\partial x)_{E_i}$. The boundary $\psi$-field is obtained through central averaging, $\psi_{E_{ij}} = (\psi_{ij} + \psi_{i+1j})/2$ and the chemical potential gradient is computed using a second-order central scheme, $(\partial\mu_\phi/\partial x)_{E_{ij}} = (\mu_{\phi_{i+1j}} - \mu_{\phi_{ij}})/\Delta x$. It should be emphasized that the fluxes are computed so that the inward flux for one cell is always equal to the outward flux of a neighbor cell, e.g. $F_{N_{ij}} = -F_{S_{ij+1}}$.

At each time step, the discrete phase fields are updated through a first-order Euler scheme,

$$\phi_{ij}^{n+1} = \phi_{ij}^n + \frac{\Delta t}{V_{ij}} \sum_{k_{ij}} (F_{Ak_{ij}} + F_{Dk_{ij}}) \tag{S11}$$

### 1.3 Thermodynamic force

The coupling between the phase-field dynamics and the hydrodynamics relies on the thermodynamic force $\boldsymbol{F} = -\phi\nabla\mu_\phi - \psi\nabla\mu_\psi$ (equations (6a) and (6b)), which is computed using central second-order finite-difference schemes. The discrete calculation of $\boldsymbol{F}$ is known to be related to the emergence of *spurious currents* in the flow[5]. Simulations have been carefully checked in order to avoid significant interactions between the spurious currents and the phase-separation dynamics. In some rare cases, it has been noted that long-term spurious forces can result in a global velocity drift of the system through the periodic domain. As large spurious velocity drifts may deteriorate the accuracy and stability of the simulated phase-field dynamics, this effect has been systematically avoided by discarding the space-averaged part of the thermodynamic force at each time step.

## 2 Data analysis

### 2.1 $\phi$-field domain size, $\lambda$

The characteristic domain size $\lambda$ is determined using the circular averaged structure factor $S(k,t) = \langle F[\phi_w](\boldsymbol{k},t), F[\phi_w](-\boldsymbol{k},t)\rangle_k$, where $F[\phi]$ is the two-dimensional Fourier transform of the windowed $\phi$-field $\phi_w = (1-\psi)\phi$, $k$ is the modulus of the wave vector $\boldsymbol{k}$ and $\langle\ \rangle_k$ is a circular averaging operator in the wave vector space defined by the radius $k$. The wavelength is then defined as[5]

$$\lambda = 2\pi \frac{\int S(k,t)dk}{\int kS(k,t)dk}. \tag{S12}$$

### 2.2 Number of inner phase domains, $N_D$

The number of $\phi$-field phase domains is automatically calculated during the simulations. A phase domain is defined as a series of neighboring computational nodes with the same value of $\phi/|\phi|$ (i.e. same sign of $\phi$). Neighbor nodes include the east, west, north and south nodes but also the diagonal ones. Phase domains are only considered in the inner droplet region, defined as $\psi < 0.5$.

### 2.3 Droplet elongation, $E$

The droplet interface position is computed systematically during the simulations. Rays are drawn from the droplet barycenter for a series of angles. For each angle $\theta$, the interface position $r(\theta)$ is defined as $\psi = 0.5$ and computed through linear interpolation. The interface deviation is defined as $\delta(\theta) = L/2 - r(\theta)$ and the droplet elongation reads

$$E = F_2 \left[ \frac{2\delta(\theta)}{L} \right], \tag{S13}$$

where $F_2$ denotes the amplitude of the second Fourier mode, obtained through fast Fourier transform.

### 2.4 Phase domain aspect ratio

Phase domain aspect ratios are quantified in figure 4(i) to analyze the transient "croissant" states of the droplets. To determine the aspect ratio of a given domain, we construct for each angle $\theta \in [0, \pi]$ a pair of perpendicular lines through the domain barycenter, where $\theta$ is the angle between one of the two lines and the $x$ axis. The lengths $h(\theta)$ and $w(\theta)$ are defined by the cross section of each of these lines with the domain area, respectively. The domain aspect ratio $h/w$ is then defined as the maximum ratio $h(\theta)/w(\theta)$ across all angles $\theta$.

Aspect ratios are averaged over series of snapshots where $N_D = 5$, and over a series of 25 simulations. Phase domains and their neighbors are determined following the same approach as for the computation of $N_D$, and only the domains with 2 neighbors are included in the averaging.

## 3 Domain aspect ratio for infinite chain

Here we derive for an infinite chain of equally sized domains the domain aspect ratio in mechanical equilibrium (Fig. S1a). In mechanical equilibrium, the outer interfaces will be circular arcs. Moreover,

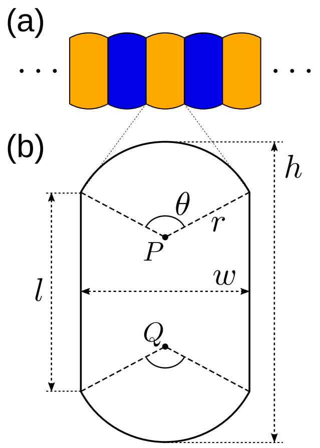


Figure S1: Sketch to compute the domain aspect ratio $h/w$.

with equal outer surface tension $\sigma_o := \sigma_{13} = \sigma_{23}$ and equal domain sizes, the inner interfaces will be straight. With the inner surface tension $\sigma_i = \sigma_{12}$, the surface tension energy per domain is

$$E = \sigma_i l + 2\sigma_0 r\theta. \tag{S14}$$

Here, the quantities $l, r, \theta$ are defined as indicated in Fig. S1b. Note that inner interfaces are shared with adjacent domains, so that each of the two inner interfaces contributes $\sigma_i l/2$ to the energy $E$ per domain.

To obtain the domain aspect ratio, we need to minimize the energy $E$ under the constraint of constant domain area $A$, which is:

$$A = wl + r^2\theta - wr\cos\left(\tfrac{\theta}{2}\right), \tag{S15}$$

where the domain width is

$$w = 2r\sin\left(\tfrac{\theta}{2}\right). \tag{S16}$$

To minimize the energy $E$, we vary it using a constant area constraint, $A = A_0$, with the pressure $p$ as Lagrange multiplier:

$$0 = \delta\Big(E - p[A - A_0]\Big), \tag{S17}$$

where the variations $\delta l, \delta r, \delta\theta$ are independent of each other. This results in the following relations:

$$\sigma_i = 2pr\sin\left(\tfrac{\theta}{2}\right) \qquad \text{from variation of } l, \tag{S18}$$

$$\theta\Big[\sigma_o - pr\Big] = p\Big[l - 2r\cos\left(\tfrac{\theta}{2}\right)\Big]\sin\left(\tfrac{\theta}{2}\right) \qquad \text{from variation of } r, \tag{S19}$$

$$2\Big[\sigma_o - pr\Big] = p\Big[l - 2r\cos\left(\tfrac{\theta}{2}\right)\Big]\cos\left(\tfrac{\theta}{2}\right) \qquad \text{from variation of } \theta. \tag{S20}$$

The first equation, Eq. (S18), can be transformed into (using Eq. (S16)):

$$\sigma_i = pw. \tag{S21}$$

This corresponds to vertical force balance across a horizontal line through the middle of the domains.

From Eqs. (S19) and (S20) with $\theta > 0$ follows that

$$\sigma_o = pr, \tag{S22}$$

$$l = 2r\cos\left(\tfrac{\theta}{2}\right). \tag{S23}$$

This is because if one of the two Eqs. (S22) and (S23) did not hold, then Eqs. (S19) and (S20) would imply that $\theta/2 = \tan(\theta/2)$ whose only solution in the range $[0, \pi/2)$ is $\theta = 0$. Note that Eq. (S22) corresponds to the Laplace pressure equation for the curved external domain boundary. Furthermore, Eq. (S23) implies that the centers of the two circular arcs, $P$ and $Q$ in Fig. S1b, coincide: $P \equiv Q$. Hence, the domain height corresponds to the circle diameter:

$$h = 2r. \tag{S24}$$

With this, we finally obtain for the aspect ratio:

$$\frac{h}{w} = \frac{2r}{w} = \frac{2\sigma_o}{\sigma_i} = \frac{2}{Ca}. \tag{S25}$$

Here, in the first step we used Eq. (S24), in the second step we used Eqs. (S22) and (S21), and in the third step we used that $Ca$ for equal surface tensions is $Ca = \sigma_i/\sigma_o$.

As an alternative derivation, one can use *horizontal* force balance across a *vertical* line through the middle of a domain, which reads:

$$2\sigma_o = ph. \tag{S26}$$

Combined with Eq. (S21), i.e. *vertical* force balance across a *horizontal* line through the middle of the domains, this yields Eq. (S25).

## References


[1] T. Krüger, H. Kusumaatmaja, A. Kuzmin, O. Shardt, G. Silva and E. M. Viggen, *Springer International Publishing*, 2017, **10**, 4–15.

[2] D. d'Humières and I. Ginzburg, *Computers & Mathematics with Applications*, 2009, **58**, 823–840.

[3] S. Gsell, U. D'Ortona and J. Favier, *Journal of Computational Physics*, 2021, **429**, 109943.

[4] Z. Guo, C. Zheng and B. Shi, *Physical Review E*, 2002, **65**, 046308.

[5] A. Tiribocchi, N. Stella, G. Gonnella and A. Lamura, *Physical Review E*, 2009, **80**, 026701.
